# Supplementary material for: Seal-3D: Interactive Pixel-Level Editing for Neural Radiance Fields
Source: arXiv:2307.15131 source file (2023-08-27)
Supplement: Supplementary file 1 [file supp.tex]

\section{Details of Editing Proxy Functions}

\subsection{Anchor Tool}

The anchor tool stretches a control point $\mathbf{x}^c$ along a translation vector $\mathbf{t}$, with its surrounding region. The translation function is defined as $\mathrm{stretch}(\cdot;\mathbf{x}^c, \mathbf{t})$. We describe the mapping function for the anchor tool as follows in the main paper:

\begin{equation}
\begin{aligned}
    % \msymbol{point_pos}^m & =\msymbol{point_pos} + growth(\msymbol{point_pos}, \Vec{t})\\
    \msymbol{point_pos}^{s} &= \mathrm{stretch}^{-1}(\msymbol{point_pos}^{t};\mathbf{x}^c, \mathbf{t}) \\
    \msymbol{mapper_func} & \defeq (\msymbol{point_pos}^{t}, \msymbol{point_dir}^{t}) \mapsto (\msymbol{point_pos}^{s}, \msymbol{point_dir}^{t})
\end{aligned}\notag
\end{equation}

% \begin{figure}[h!]
% \centering
%     \includegraphics[width=\linewidth, clip, trim=0 0px 0 0]{resources/supp/supp-anchor.pdf}
%     % \vspace{-2em}
% \caption{}
% \label{fig-anchor-detail}
% % \vspace{-1.5em}
% \end{figure}

% As we only care about the mapping function $\mathrm{stretch}^{-1}$ in implementation, we are not to explain its positive version $\mathrm{stretch}$. 

As \cref{fig-anchor-detail} shows, the mapping function $\mathrm{stretch}^{-1}$ is realized by projecting a point $\mathbf{x}^t$ in the target conic space  $\mathcal{T}$ (blue)  to the source space $\mathcal{S}$ (green). The detailed steps are as follows.

\begin{figure}[h]
    \centering
    \setlength{\tabcolsep}{5pt}
    % \vspace{-1em}
    \resizebox{\columnwidth}{!}{
    \begin{tabular}{ccc}
        \includegraphics[width=2.5cm,clip]{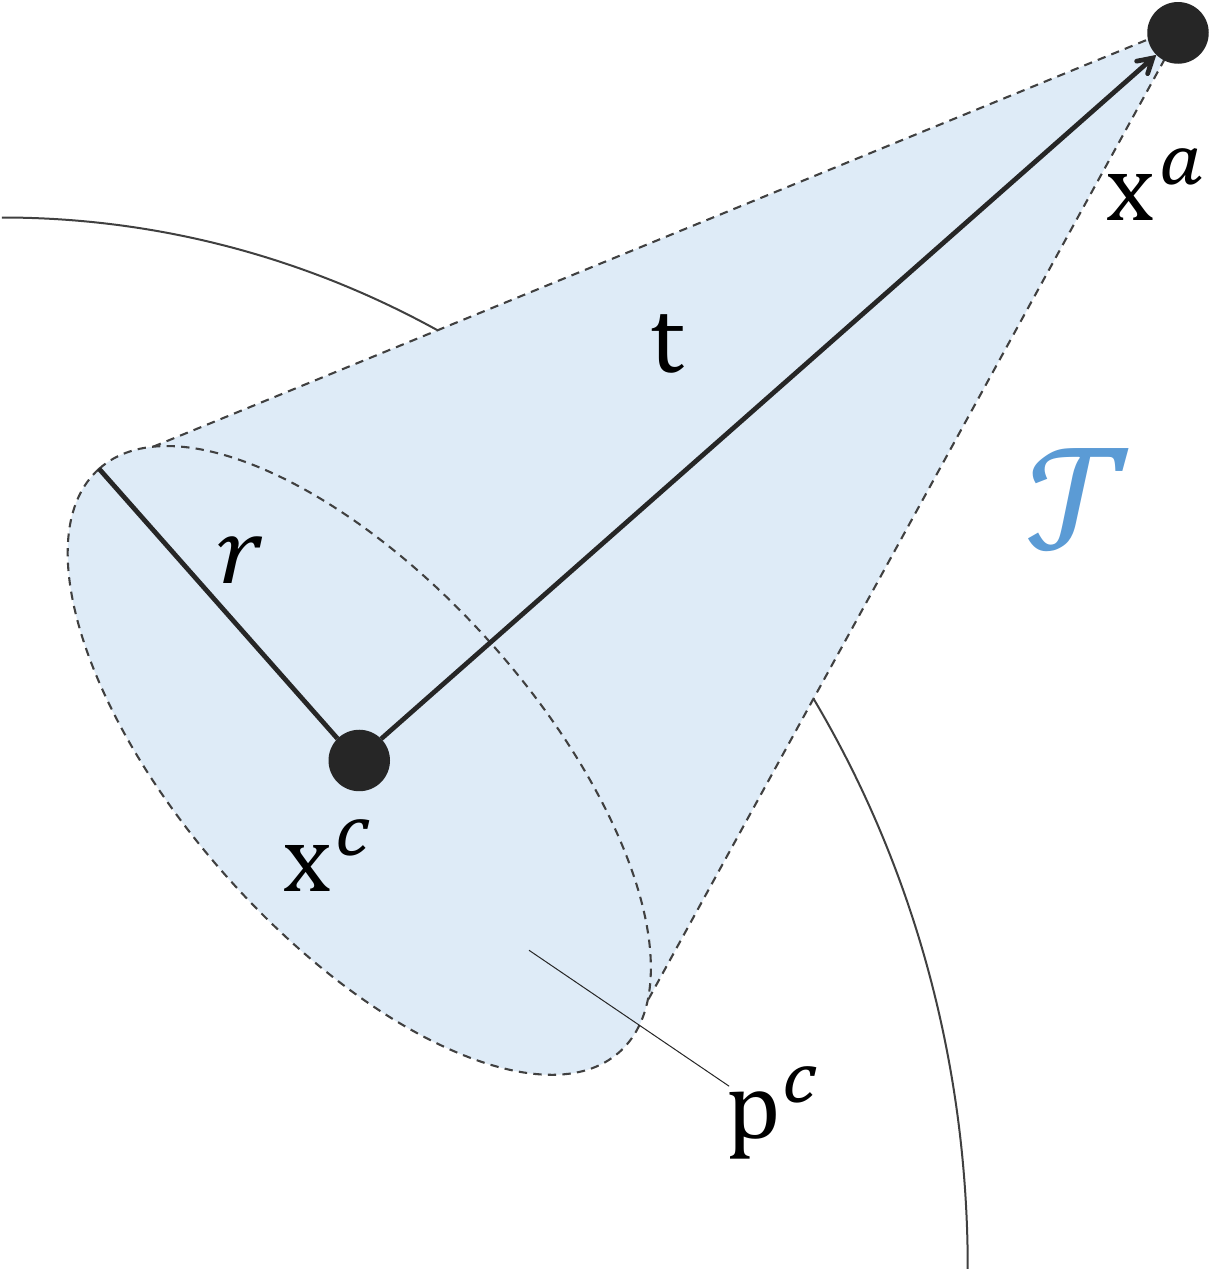} & \includegraphics[width=2.5cm,clip]{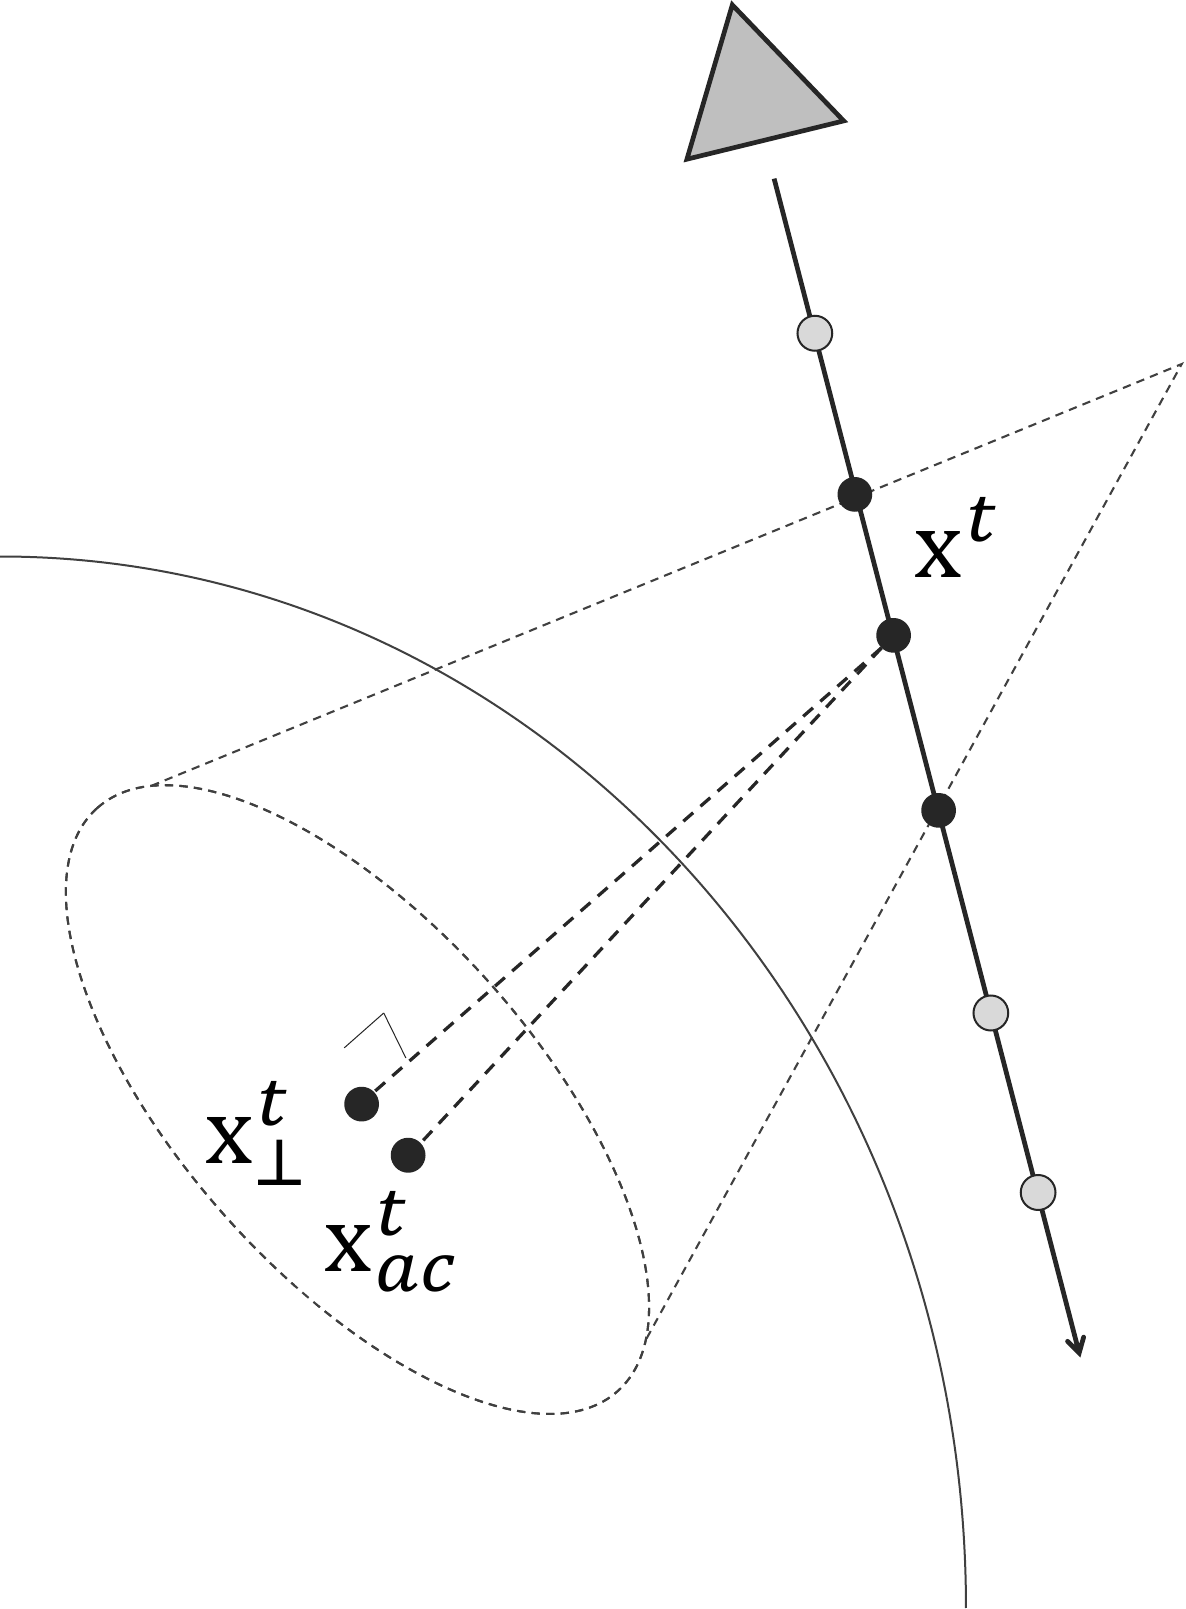} &
        \includegraphics[width=2.5cm,clip]{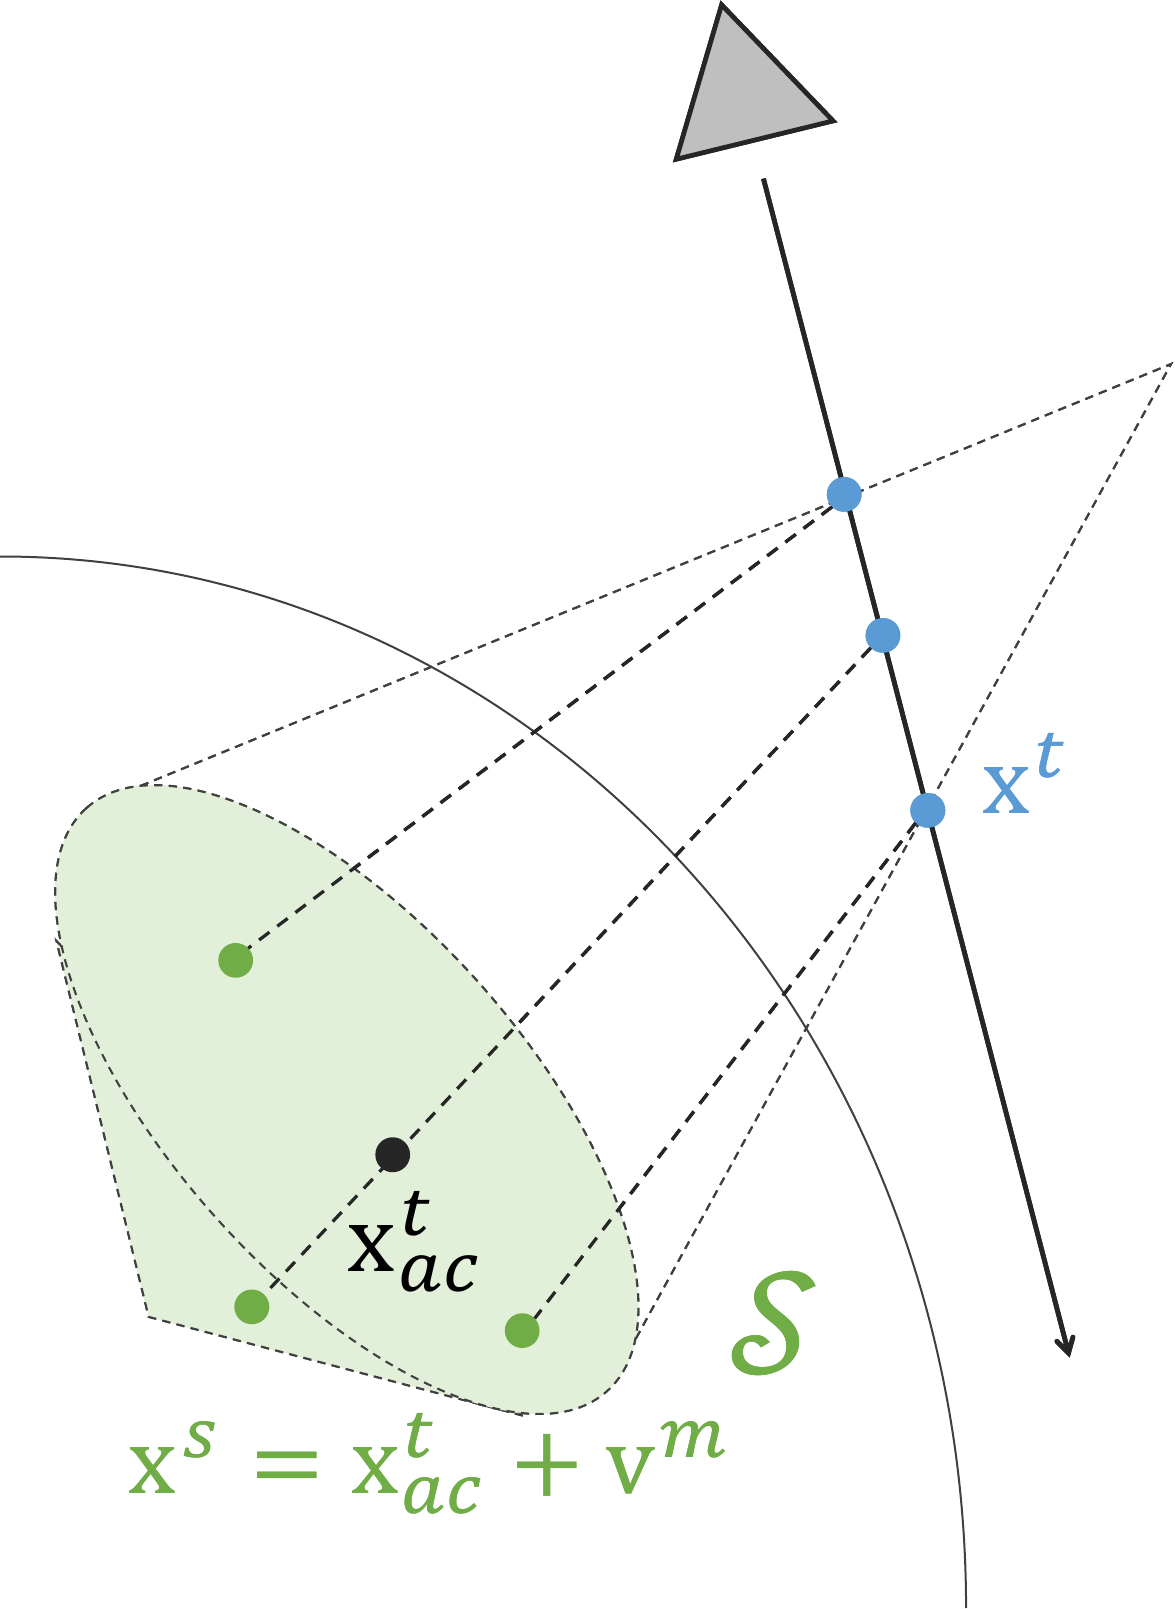}\\
        (a) Construct $\mathcal{T}$ & (b) Find $\mathbf{x}^t$ in $\mathcal{T}$ & (c) Translate $\mathbf{x}^t$ to $\mathbf{x}^s$  \\
    \end{tabular}
    }
    % \vspace{-0.5em}
    \caption{The details of the anchor tool's mapping function. $\mathcal{T}$ (blue) is mapped to $\mathcal{S}$ (green) to make sure $\mathbf{x}^t$ on the surface of the cone are mapped to the surface of the object, while $\mathbf{x}^t$ inside the cone are mapped to the inner space of the object.}
    % \vspace{-1em}
    \label{fig-anchor-detail}
    % \vspace{-0.5em}
\end{figure}

\begin{enumerate}
\item Construct the target conic space $\mathcal{T}$. The base of the cone is a circle with radius $r$ defined by user input on a plane $\mathbf{p}^c$ where the control point $\mathbf{x}^c$ is on. We search the surface points $\mathbf{x}^p$ near $\mathbf{x}^c$ and fit the $\mathbf{p}^c$ from $\mathbf{x}^p$ using SVD decomposition and least-squares fitting. The point $\mathbf{x}^a = \mathbf{x}^c + \mathbf{t}$ is the apex of the cone.

\item Find $\mathbf{x}^{t}$ that are inside $\mathcal{T}$. Here we define the projected point from $\mathbf{x}^{t}$ to $\mathbf{p}^c$ as $\mathbf{x}^{t}_{\perp}$, the  projected point from $\mathbf{x}^a$ to $\mathbf{p}^c$ as $\mathbf{x}^{a}_{\perp}$, and the  projected point from $\mathbf{x}^{t}$ to $\mathbf{p}^c$ along direction of the vector $\overrightarrow{\mathbf{x}^a\mathbf{x}^c}$ as $\mathbf{x}^{t}_{ac} = \mathbf{x}^{t} + \frac{|\overrightarrow{\mathbf{x}^{t}\mathbf{x}^{t}_{\perp}}|}{|\overrightarrow{\mathbf{x}^a\mathbf{x}^a_{\perp}}|}\cdot\overrightarrow{\mathbf{x}^a\mathbf{x}^c}$. The conditions are as follows:

\begin{align}
    \overrightarrow{\mathbf{x}^{t}_\perp\mathbf{x}^{t}}\cdot\overrightarrow{\mathbf{x}^a_\perp\mathbf{x}^a} &> 0\label{eq-anchor-filter-side}\\
    |\overrightarrow{\mathbf{x}^c\mathbf{x}^{t}_{ac}}| &< r\label{eq-anchor-filter-radius}\\
    |\overrightarrow{\mathbf{x}^{t}\mathbf{x}^{t}_{\perp}}| &< |\overrightarrow{\mathbf{x}^a\mathbf{x}^a_{\perp}}|\label{eq-anchor-filter-height}\\
    \frac{|\overrightarrow{\mathbf{x}^{t}\mathbf{x}^{t}_{ac}}|}{|\overrightarrow{\mathbf{x}^c\mathbf{x}^{t}_{ac}}|} &< \frac{|\overrightarrow{\mathbf{x}^a\mathbf{x}^c}|}{r}\label{eq-anchor-filter-cone}
\end{align}\notag

\item Translate $\mathbf{x}^{t}$ to $\mathbf{x}^{s}$. The mapping function is defined as follows, where $w^m$ is the weight of the $\mathbf{x}^a\mathbf{x}^c$ direction offset vector $\mathbf{v}^m$, which is designed to monitor the surface thickness. In our implementation, we set $w^m$ to $0.1$.
% \begin{scriptsize}
\begin{align}
    &\mathbf{v}^m = - w^m \cdot\frac{|\overrightarrow{\mathbf{x}^a\mathbf{x}^c}|-|\overrightarrow{\mathbf{x}^{t}\mathbf{x}^{t}_{ac}}|}{|\overrightarrow{\mathbf{x}^a\mathbf{x}^c}|}\cdot\mathbf{x}^a\mathbf{x}^c\\
    &\mathrm{stretch}^{-1}(\msymbol{point_pos}^{t};\mathbf{x}^c, \mathbf{t})=\left\{
        \begin{array}{ll}
            \mathbf{x}^{t}_{ac} + \mathbf{v}^m&,\text{if \cref{eq-anchor-filter-side,eq-anchor-filter-radius,eq-anchor-filter-height,eq-anchor-filter-cone}}\\
            \mathbf{x}^{t}&,\text{otherwise}
        \end{array}
        \right.
\end{align}
% \end{scriptsize}
\end{enumerate}

\subsection{Color Tool}

The color tool transfers the color of the target space. To preserve shading details, we first convert the color in RGB space to HSL or HSV color space, modify the lightness (L of HSL) or value (V of HSV), and convert the modified color back to RGB space. Take the HSL color space as an example, we keep the value of hue (H) and saturation (S) from the modification color $c^m$ and offset the lightness (L) of $c^m$ using the lightness of the original color $c^o$. Here we define the function $\mathrm{RGB2HSL}$ as a conversion from RGB space to HSL space and the function $\mathrm{HSL2RGB}$ as a conversion from HSL space to RGB space. The mapped color $c^t$ is computed as follows:

\begin{align}
    &[h^m, s^m, l^m] = \mathrm{RGB2HSL}(c^m)\notag\\
    &[h^o, s^o, l^o] = \mathrm{RGB2HSL}(c^o)\notag\\
    &c^t = \mathrm{HSL2RGB}([h^m, s^m, l^m + l^o-\mathrm{mean}(l^o))])
\end{align}

Color modification with HSV color space is similar to HSL, while the lightness (L) is replaced with the value (V).

\section{Teacher Model Output \textit{v.s} Local Pertaining in Fast Preview}

Local pretraining is proposed for the fast preview. Using the teacher model output for preview could be a bottleneck of speed during preview, giving a rendering speed of only 1-2 FPS when the editing space is very large and the sampling-computing-mapping operations of the proxy function become extremely complicated, much slower than the NGP rendering speed at 20-30 FPS, making it not practical for interactive preview.

\section{Additional Results}
Additional results are shown in \cref{fig-additional-1,fig-additional-2,fig-additional-3,fig-additional-4}.

~\\

\begin{figure}[H]
\centering
    \includegraphics[width=\linewidth, clip, trim=0 0px 0 0]{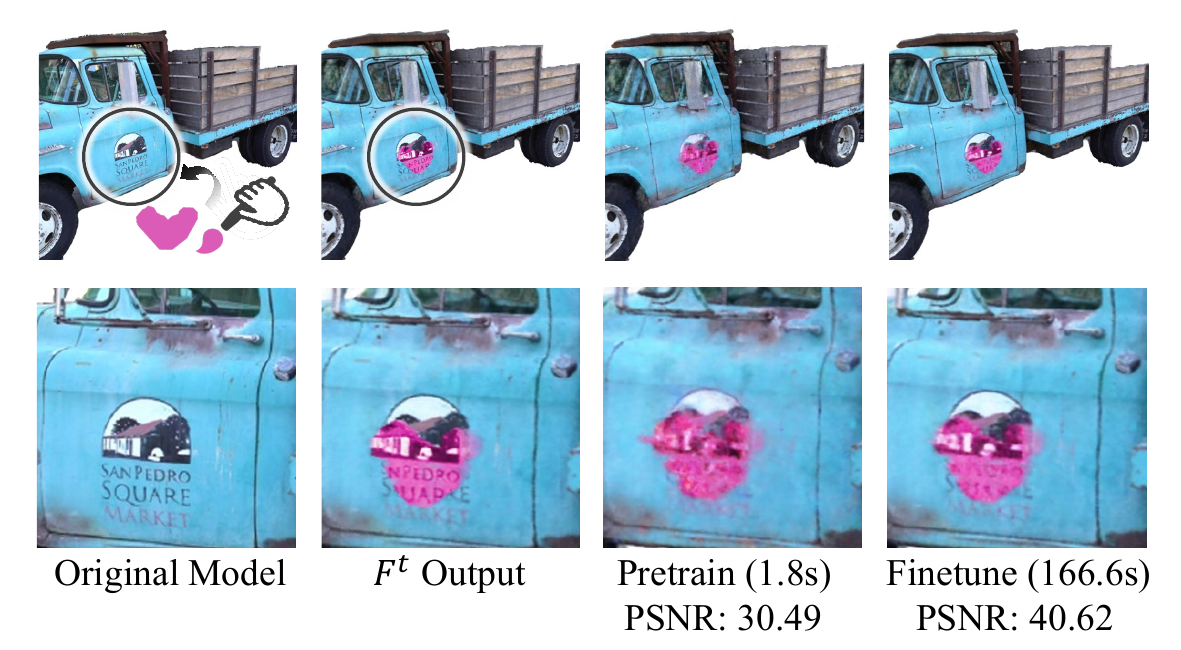}
    \vspace{-2em}
\caption{\small{Example of color and brush editing on the real-world scene: paint a pink heart on the truck (Tanks and Temples\cite{Knapitsch2017}).}}
\label{fig-additional-1}
\vspace{-1em}
\end{figure}

\begin{figure}[H]
\centering
    \includegraphics[width=\linewidth, clip, trim=0 0px 0 0]{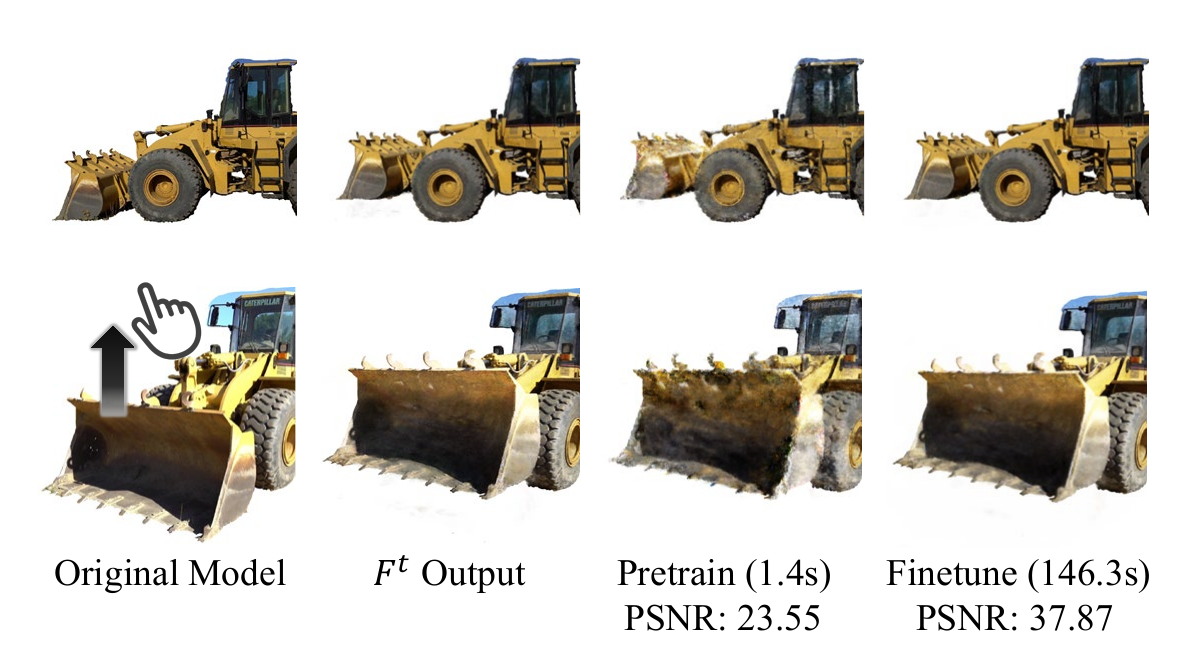}
    \vspace{-2em}
\caption{\small{Example of bounding shape editing on the real-world scene: lift the bucket of forklift (Tanks and Temples\cite{Knapitsch2017}).}}
\label{fig-additional-2}
\vspace{-1em}
\end{figure}

\begin{figure}[H]
\centering
    \includegraphics[width=\linewidth, clip, trim=0 0px 0 0]{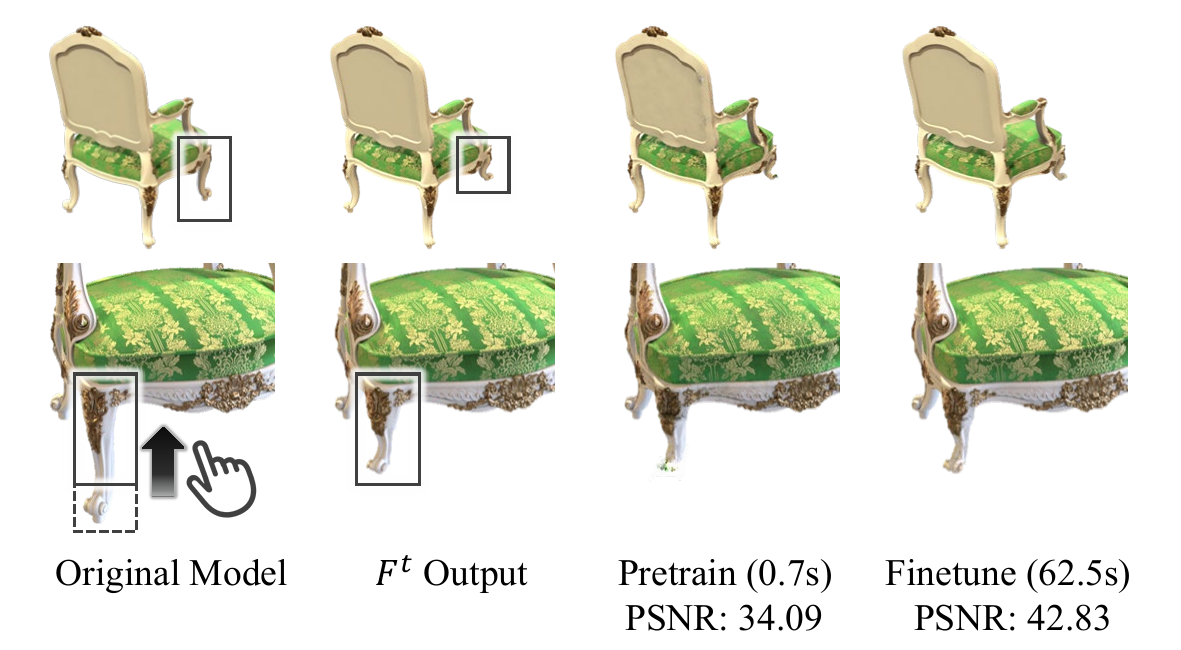}
    \vspace{-2em}
\caption{\small{Example of bounding shape editing: shrink the chair leg (NeRF Blender\cite{mildenhall2020nerf}).}}
\label{fig-additional-3}
\vspace{-1.5em}
\end{figure}

\begin{figure}[H]
\centering
    \includegraphics[width=\linewidth, clip, trim=0 0px 0 0]{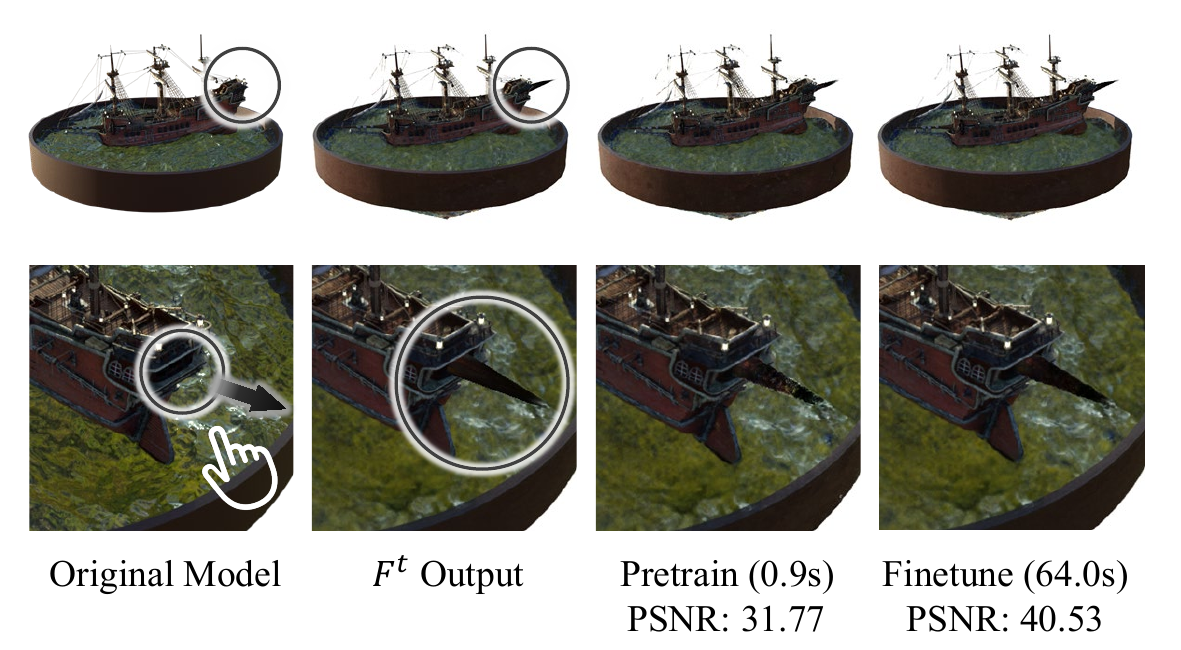}
    \vspace{-2em}
\caption{\small{Example of anchor editing: fake bowsprit of the ship (NeRF Blender\cite{mildenhall2020nerf}).}}
\label{fig-additional-4}
\vspace{-1em}
\end{figure}
